# Supplementary material for: Non-Relational Databases on FPGAs: Survey, Design Decisions, Challenges
Source: arXiv:2007.07595 source file (2020-07-15)
Supplement: Supplementary file 1 [file appendix.tex]

\newpage
\appendix

\section{Old stuff}

\subsection{Operator}
Archetypes: PEs, pipeline steps

\subsection{Binary Representation}
Hard to separate from memory access.
%TODO Double check again if all papers are correctly assigned

GraphChi seems to be The competitor for disk based CPU graph processing and is what most representations seem to be based on. 

Graph archetypes: Partitioning, compression, graph as dynamic circuit in hardware

\subsection{Dynamic Queries}
Archetypes: Partial reprogramming or configuration parameters in BRAM or PEs with instruction set / skeleton automaton

\subsection{Transactions}
This means transactions and concurrency control.

\begin{figure}[ht]
	\centering
	\includegraphics[width=0.6\linewidth]{figures/locking}
	\caption{Locking archetype.}
	\label{fig:locking}
\end{figure}

Figure \ref{fig:locking} shows the locking archetype. Work items go into the orchestrator, which routes them to the respective PE. PEs work with work item and request new (read or write) work items from the memory lock manager. The manager applies the lock and sends a request to the memory, which is routed to the work item orchestrator.

\subsection{CPU-FPGA Coalescence}
Archetypes?: Shared memory region with job queue and tables, \gls{fpga} in CPU-storage path, CPU and \gls{fpga} working at the same time on partitioned task

\subsection{Memory Access}
Archetypes: Batching/sequentializing random memory accesses, prefetching, many parallel memory requests, decoupling compute and memory access

Graph archetypes: cache with high degree vertices, building on-chip data structures for sequential access

Nothing about how to use multiple memory banks most effectively? Benchmark?

\subsection{Programming Model}

\begin{table*}[t]
\centering
\tiny
\begin{tabular}{l c r l r r r r l r r}
 \multirow{2}{*}{Framework}	& \multirow{2}{*}{Type}	& \multirow[r]{2}{*}{Bandw.(GB/s)}	& \multirow{2}{*}{Algorithm}	& \multicolumn{4}{c}{Resource Utilization}	& \multirow{2}{*}{Data Set}	& \multirow[r]{2}{*}{Perf.(MTEPS)} & \multirow[r]{2}{*}{Perf./Bandw.}	\\
 	& 	& 	& 	& \#LUTs	& \#Registers	& BRAM(MB)	& Clock(MHz)	& 	& 	&  \\
 \hline
 \multirow{4}{*}{HitGraph \cite{journals/tpds/ZhouKPSW19}}	& \multirow{4}{*}{E}	& \multirow{4}{*}{60}	& \multirow{2}{*}{PageRank}	& \multirow{2}{*}{408,993}	& \multirow{2}{*}{313,501}	& \multirow{2}{*}{9.4}	& \multirow{2}{*}{200}	& Twitter	& 2487	& 41.45 \\
 	& 	& 	& 	& 	& 	& 	& 	& LiveJournal	& 2110	& 35.17 \\
 	& 	& 	& \multirow{2}{*}{WCC}	& \multirow{2}{*}{207,199}	& \multirow{2}{*}{181,374}	& \multirow{2}{*}{9.1}	& \multirow{2}{*}{200}	& Twitter	& 3395	& 56.58 \\
 	& 	& 	& 	& 	& 	& 	& 	& LiveJournal	& 3322	& 55.37 \\
 \hline
 \multirow{6}{*}{ForeGraph \cite{conf/fpga/DaiHCXWY17}}	& \multirow{6}{*}{V}	& \multirow{6}{*}{19.2}	& \multirow{2}{*}{PageRank}	& \multirow{2}{*}{358,796}	& \multirow{2}{*}{442,587}	& \multirow{2}{*}{13.3}	& \multirow{2}{*}{187}	& Twitter	& 464	& 24.17 \\
 	& 	& 	& 	& 	& 	& 	& 	& LiveJournal	& 1193	& 58.54 \\
 	& 	& 	& \multirow{2}{*}{WCC}	& \multirow{2}{*}{385,652}	& \multirow{2}{*}{423,251}	& \multirow{2}{*}{13.3}	& \multirow{2}{*}{173}	& Twitter	& 432	& 22.5 \\
 	& 	& 	& 	& 	& 	& 	& 	& LiveJournal	& 1124	& 58.54 \\
 	& 	& 	& \multirow{2}{*}{BFS}	& \multirow{2}{*}{335,163}	& \multirow{2}{*}{371.687}	& \multirow{2}{*}{14.8}	& \multirow{2}{*}{205}	& Twitter	& 364	& 18.96 \\
 	& 	& 	& 	& 	& 	& 	& 	& LiveJournal	& 1069	& 55.68 \\
 %\hline
 %\multirow{4}{*}{Graphicionado \cite{DBLP:conf/micro/HamWSSM16}}	& \multirow{4}{*}{V}	& \multirow{4}{*}{68}	& \multirow{2}{*}{PageRank}	& \multirow{2}{*}{-}	& \multirow{2}{*}{-}	& \multirow{2}{*}{64}	& \multirow{2}{*}{1000}	& Twitter	& (4500) \\
 % 	& 	& 	& 	& 	& 	& 	& 	& LiveJournal	& (4600) \\
 %	& 	& 	& \multirow{2}{*}{BFS}	& \multirow{2}{*}{-}	& \multirow{2}{*}{-}	& \multirow{2}{*}{64}	& \multirow{2}{*}{1000}	& Twitter	& (1000) \\
 %	& 	& 	& 	& 	& 	& 	& 	& LiveJournal	& (1500) \\
 %\hline
 %\multirow{2}{*}{GraphVF \cite{DBLP:conf/fpl/EngelhardtS16}}	& \multirow{2}{*}{V}	& \multirow{2}{*}{20.2}	& PageRank	& 113776	& 80074	& 4.9	& 125	& -	& (3000) \\
 %	& 	& 	& BFS	& 39986	& 21502	& 2.9	& 125	& -	& (3000) \\
 \hline
 \multirow{2}{*}{Zhang \cite{DBLP:conf/fpga/ZhangL18}}	& \multirow{2}{*}{BFS}	& \multirow{2}{*}{(HMC) 60}	& \multirow{2}{*}{BFS}	& \multirow{2}{*}{113776}	& \multirow{2}{*}{-}	& \multirow{2}{*}{4.9}	& \multirow{2}{*}{125}	& RMAT(24,16)	& 36900	& 615 \\
 	& 	& 	& 	& 	& 	& 	& 	& RoadNet USA	& 400	& 6.67 \\
\end{tabular}
\caption{Graph Processing Frameworks.}
\label{tab:frameworks}
\end{table*}

Often comes with performance model.

Archetypes: User defined functions/kernels in predefined template operators that are chained (can be described with higher language / library vs framework?), (state machines)

Graph archetypes: 
\begin{enumerate}
	\item Access pattern: Vertex-centric(gather apply scatter), edge-centric
	\item Traversal pattern: Breadth first search
	\item Algorithm: ...
	\item Implementation: Semi-ring
	\item Partitioning: Interval-shard model
\end{enumerate}

\subsection{Performance Model}
Archetypes: Modelling memory bandwidth with packet model or modelling problem specific parallelism vectors with constraints

Archetype: Modelling upper bound of performance (throughput) by exploring parallelism dimensions with resource constraints

Possible measures (graph): traversed edges per second

\section{Old stuff 2}

\subsubsection{Operator}

\todo[inline]{Pipelining and Replication can be combined arbitrarily}

\paragraph{SIMD \cite{conf/pdpta/TakeiHK14}}

\paragraph{Item Level Pipelining \cite{conf/hpcc/LiuZJJ19} (\cite{conf/ipps/BondhugulaDFWS06, journals/tjs/MilovanovicMBT07, conf/fpga/DaiNZ10, conf/fpl/LiangYKW16})}
Pipelining on \glspl{fpga} is one form of parallelism. 
When algorithms are split up into pipelines, all pipeline stages can be executed in parallel. 
The latency might rise with pipelining, but pipelining can also hide latency. 
This is only possible on \glspl{fpga} (CPUs only support limited, rigid instruction pipelining).

\paragraph{Kernelization \cite{DBLP:conf/fpga/ZhangKL17, DBLP:conf/fpga/ZhangL18, DBLP:conf/fpl/UmurogluMJ15, conf/hpcc/LiuZJJ19}} 
Identification of simplifying kernels or kernels that perform well in certain situations. 
An example are the top down and bottom up kernels of breadth first search, which can form a hybrid approach, where one kernel is selected in each iteration of the algorithm. 
This can be problematic on \glspl{fpga} since it needs additional resources to deploy multiple kernels.

\paragraph{Task Level Pipelining \cite{conf/fpl/LiangYKW16}}

\paragraph{Replication}

\paragraph{Datapath \cite{conf/ipps/BondhugulaDFWS06, journals/tjs/MilovanovicMBT07, journals/tcas/LeiDLX16, DBLP:conf/fpt/WangJXP10, conf/ipps/AttiaJTJZ14, journals/iracst/LeiRG15, DBLP:conf/fpga/BestaFBLH19, journals/corr/abs-0909-1781}} 
Dataflow that is impossible in the rigid design of CPUs This is only possible on \glspl{fpga}. 
Network on chip? 
\cite{journals/iracst/LeiRG15} 
Systolic array

\subsubsection{Binary Representation}

\paragraph{Partitioning \cite{conf/ipps/BondhugulaDFWS06, DBLP:conf/fpt/WangJXP10, journals/iracst/LeiRG15, DBLP:conf/fpl/UmurogluMJ15, DBLP:conf/dac/FinnertySLL19}} 
Partitioning the input data can be used for multiple other optimizations. 
Partitions can be \eg worked on in parallel, used to split up data over multiple memory modules or prefetched. 
Partitioning might incur high initialization costs.

\paragraph{Sorting \cite{conf/ipps/ZhouCP15, DBLP:conf/fpga/ZhangKL17, DBLP:conf/fpga/ZhangL18}} 
Sorting the data with upfront knowledge about the dataset can lead to sequentialization of memory accesses.

\paragraph{Compression \cite{DBLP:conf/fpl/BetkaouiWTL12, conf/ipps/AttiaJTJZ14, DBLP:journals/ieiceee/NiDZLW14, DBLP:conf/fpga/ZhangKL17, DBLP:conf/fpga/ZhangL18, DBLP:conf/dac/FinnertySLL19, journals/sigarch/VanderbauwhedeFCM13}} 
Lossless data compression leads to lower bandwidth usage for the same information.

\paragraph{Parsing \cite{conf/fccm/BondhugulaDDFWSS06, conf/reconfig/El-HassanI10}} 
This is too general. Maybe rename to indexing?
Parsing in this context means transforming the data into a format that facilitates working on it in the accelerator. 
Sorting is one (maybe most?) important specialization of this.

\section{Old stuff 3}

Research gap is based on following differences between generic solutions and database requirements:
\begin{itemize}
	\item Different design (integration as co-processor, reconfigurability during runtime)
	\begin{itemize}
		\item Has to work in tandem with CPU based system \emph{(maybe covered by \gls{fpga} database literature)}
		\item Generic algorithmic solutions are designed for one shot execution
	\end{itemize}
	\item Different data structures (custom binary formats, preprocessing) \emph{(maybe covered by $<$domain$>$ database literature)}
	\begin{itemize}
		\item Generic operators take generic input, but database can prepare custom format (but also has to be editable) in memory (no parsing required)
		\item All preprocessing for operators counts towards runtime, but not necessarily in database
	\end{itemize}
	\item Database specifics (index, persistence, transactional, DB plans, snapshot isolation, concurrent users) \emph{(maybe covered by database literature)}
\end{itemize}
